# Supplementary material for: Learning the Sampling Pattern for MRI
Source: arXiv:1906.08754 source file (2020-06-22)
Supplement: Supplementary file 2 [file merge_main_supp.tex]

\documentclass{article}% or something else
\usepackage{pdfpages}
\begin{document}
\includepdf[pages=-]{main}
\includepdf[pages=-]{supp_material}

\end{document}
